# Supplementary material for: Cascaded Diffusion Models for Neural Motion Planning
Source: arXiv:2505.15157 source file (2025-05-21)
Supplement: Supplementary file 1 [file appendix.tex]

\appendix

\section{Diffusion Models}
Diffusion models are probabilistic generative models which have seen wide-spread use across many generative machine learning tasks.
As noted in the main paper diffusion models consist of forward and backward processes.
In the forward process we progressively add noise to the true data distribution.
While in backward process we remove noise at each step. 
Formally, one concrete form of this process is the Ornstein-Ulhenbeck process, which is described by the following Stochastic Differential Equation (SDE):
\begin{align}
\label{eq:diffusion-cont-fwd}
    dX_t = -\frac{1}{2}\left(g(t) X_t \right)dt + \sqrt{g(t)}dW_t, \quad \text{for} \quad g(t) > 0,
\end{align}
where as we noted previously $X_0 \sim p_\text{data}$ is our true sample from the data distribution, 
$\left\{ W_t \right\}_{t \ge 0+}$ is a standard Wiener process (brownian motion) and
$g(t)$ is a non-decreasing weighting function.
Specifically, $g(t)$ is used to control the amount of noise corruption we want to add in the forward process. Many different choices for $g(t)$ have been explored in the literature including linear and cosine schedules.
The above forward process \eqref{eq:diffusion-cont-fwd} is simulated for a large number of diffusion 
timesteps and terminates at some marginal distribution $q(x_T)$ which is assumed to be close to the standard gaussian.
Solving the forward process SDE we get the backward process (by reversing time) from \eqref{eq:diffusion-cont-fwd}, 
which allows us to generate samples. 
% \begin{align}
%     dX_t = -g(t)\left[ \frac{X_t}{2} + \nabla_x \log p_t\left(X\right) \right]dt + \sqrt{g(t)}dW_t
% \end{align}

\section{Training Details}
\label{app:train-details}

In this section we further provide training and implementation details for our proposed approach.
We use discrete diffusion models based on the diffuser \cite{janner2022planning} architecture.
For all environments we use cascaded models of hierarchy 2 (i.e. $K = 2$).
We found this to be sufficient for the commonly used benchmark tasks we use for evaluation.
For each environment we use sub-goals that are 8 steps away from the current state.
Since \mpinetname uses adaptive sampling for its trajectories, i.e. some states are much closer than others, we make these farther states more closer to each other.
We use reference trajectory points that are 2, 4 and 6 steps away to guide the lower-level diffusion model for local refinement.
Table~\ref{app-tab:hparams-high} and Table~\ref{app-tab:hparams-low} report the training hyper-parameters we used for training each of our high-level ($K=2$) and low-level ($K=1$) models.

For evaluating the output plans we verify if each state in the plan has no collision.
However, since the planning states output from a learned model can be sparse,
naively using collision-checks for only these output states is insufficient.
This is because each state (from the planner output) can be in free space but the path between them can have
constraint violations (e.g. collisions).
Hence, we convert sparsely connected plan outputs states to densely connected set of waypoints and 
verify if each waypoint has no constraint.

% Please add the following required packages to your document preamble:
% \usepackage{booktabs}
\begin{table}[]
\centering
\begin{minipage}[t]{0.45\textwidth}
\centering
\begin{tabular}{@{}ll@{}}
\toprule
Hyper-param & Value \\ \midrule
learning rate & 1e-4 \\
warmup steps & 2000 \\
final lr & 1e-5 \\
optimizer & AdamW \\
weight decay & 1e-3 \\
diffusion time steps & 256 \\
channels & [32, 64, 128, 256, 512] \\ \bottomrule \\
\end{tabular}
\caption{Hyper-parameters for high-level diffusion model.}
\label{app-tab:hparams-high}
\end{minipage}
  \hfil
\begin{minipage}[t]{0.45\textwidth}
\centering
\begin{tabular}{@{}ll@{}}
\toprule
Hyper-param & Value \\ \midrule
learning rate & 2e-4 \\
warmup steps & 2000 \\
final lr & 1e-5 \\
optimizer & AdamW \\
weight decay & 5e-3 \\
diffusion time steps & 128 \\
channels & [32, 64, 128, 256] \\ \bottomrule \\
\end{tabular}
\caption{Hyper-parameters for low-level diffusion model.}
\label{app-tab:hparams-low}
\end{minipage}
\end{table}

\textbf{Plan Refinement:}
% Algorithm 1 and 2 details our cascaded diffusion approach and plan refinement strategy.
We note that our plan refinement algorithm does not rely on precisely finding the collision based states.
Instead, as noted in the main paper, 
we find the plan states output by the cascaded model and find a subsequence within these collision states. 
Additionally, if two sequence of states are separated by less than 3 non-collision states we merge the non-collision states together with the collision sequence to create a larger collision sequence.
Once we have the collision sequences we simply take the $M_{s}\text{'th}$ previous state from the start state of the collision sequence as the new start state.
Additionally, we take $M_{g}\text{'th}$ state from the end of the collision sequence as the new goal state.
For all our experiments we set $M_{s} = 2$ and $M_{g} = 2$.
Overall, even if there exists some noise in collision checking our algorithm should generally be robust to them.

\begin{figure}[t]
  \centering
  \includegraphics[width=.99\linewidth]{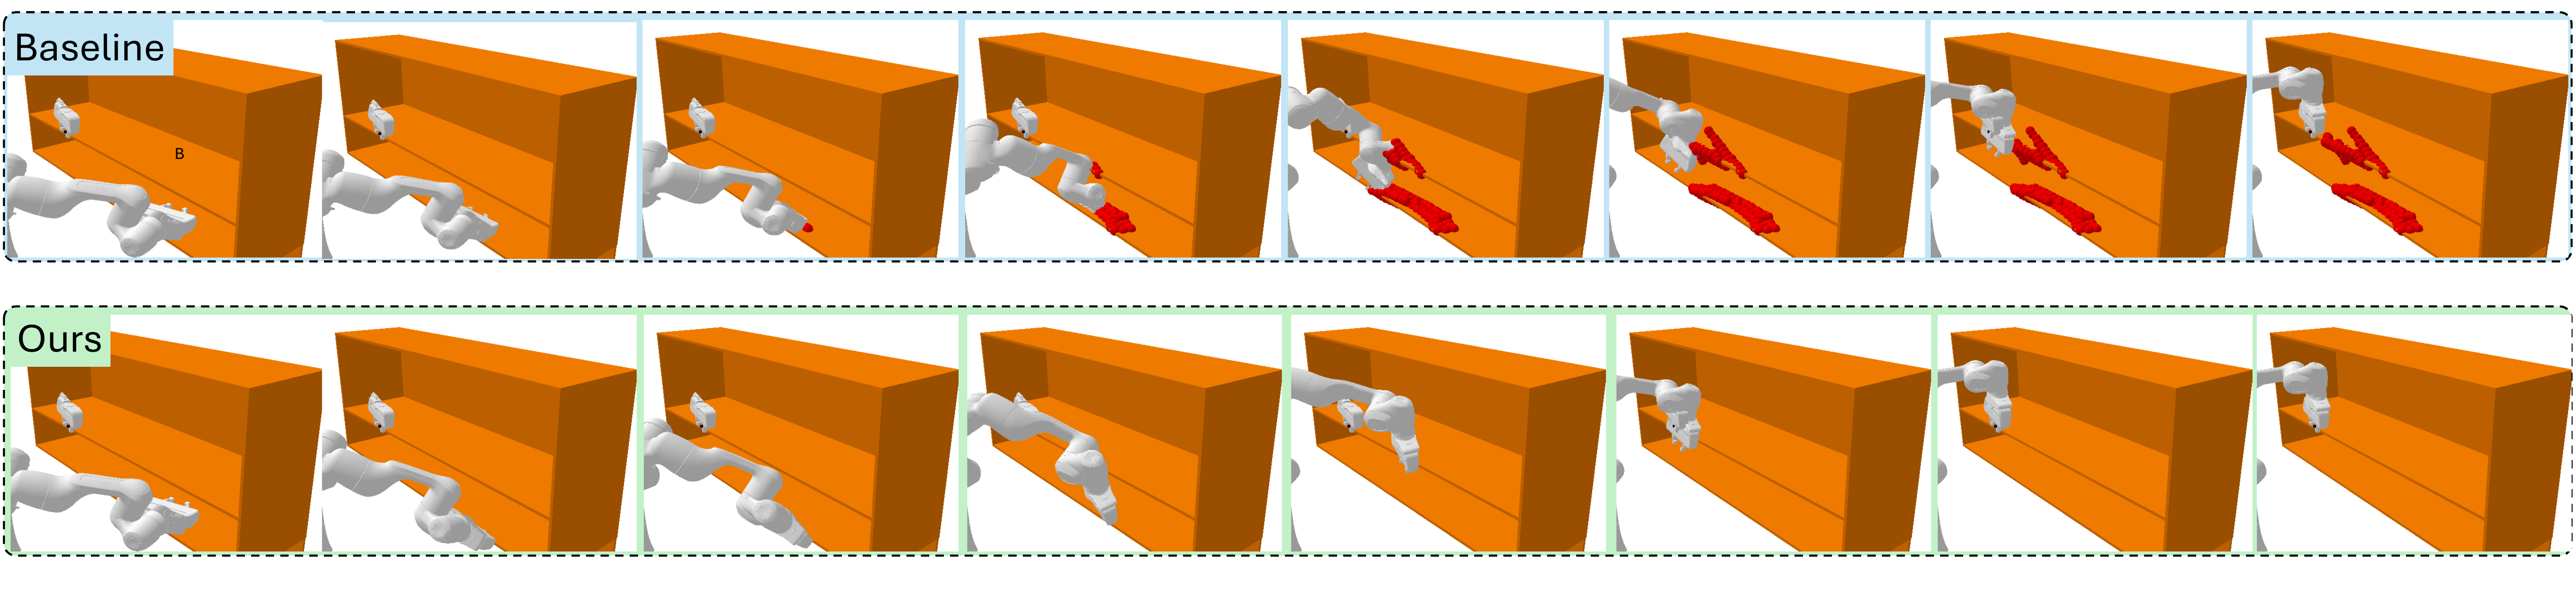} 
  \caption{\footnotesize{Qualitative results. \textcolor{red}{Red} spheres show collisions with the environment. Note that many collisions are very subtle, and the optimal solution is very close to being in collision; this is part of the difficulty of our problem setting.}}
  \label{fig:appqualitative-results}
\end{figure}

\section{Additional Results}
\label{app:ressults}

To run our plan refinement strategy we train a separate model on point cloud data to detect if the robot state is in collision with the environment. 
We generate 20000 point cloud observations both with and without collisions and train our point cloud model to output if a collision exists or not. 
To generate this data we use two sources. First, we load random point cloud scenes from our planning scene data. We also load expert configurations from the ground truth planner data.
Further, we add noise to these configurations to get collision data.
We also use configurations from our learned diffusion model (by using its generated outputs) and label it using the ground truth simulator.
Overall, we find that our collision detection model can perform quite well. We get an overall F1-score of $0.954$ for collision detection on the test set.

\begin{figure}[t]
  \centering
  \includegraphics[width=.99\linewidth]{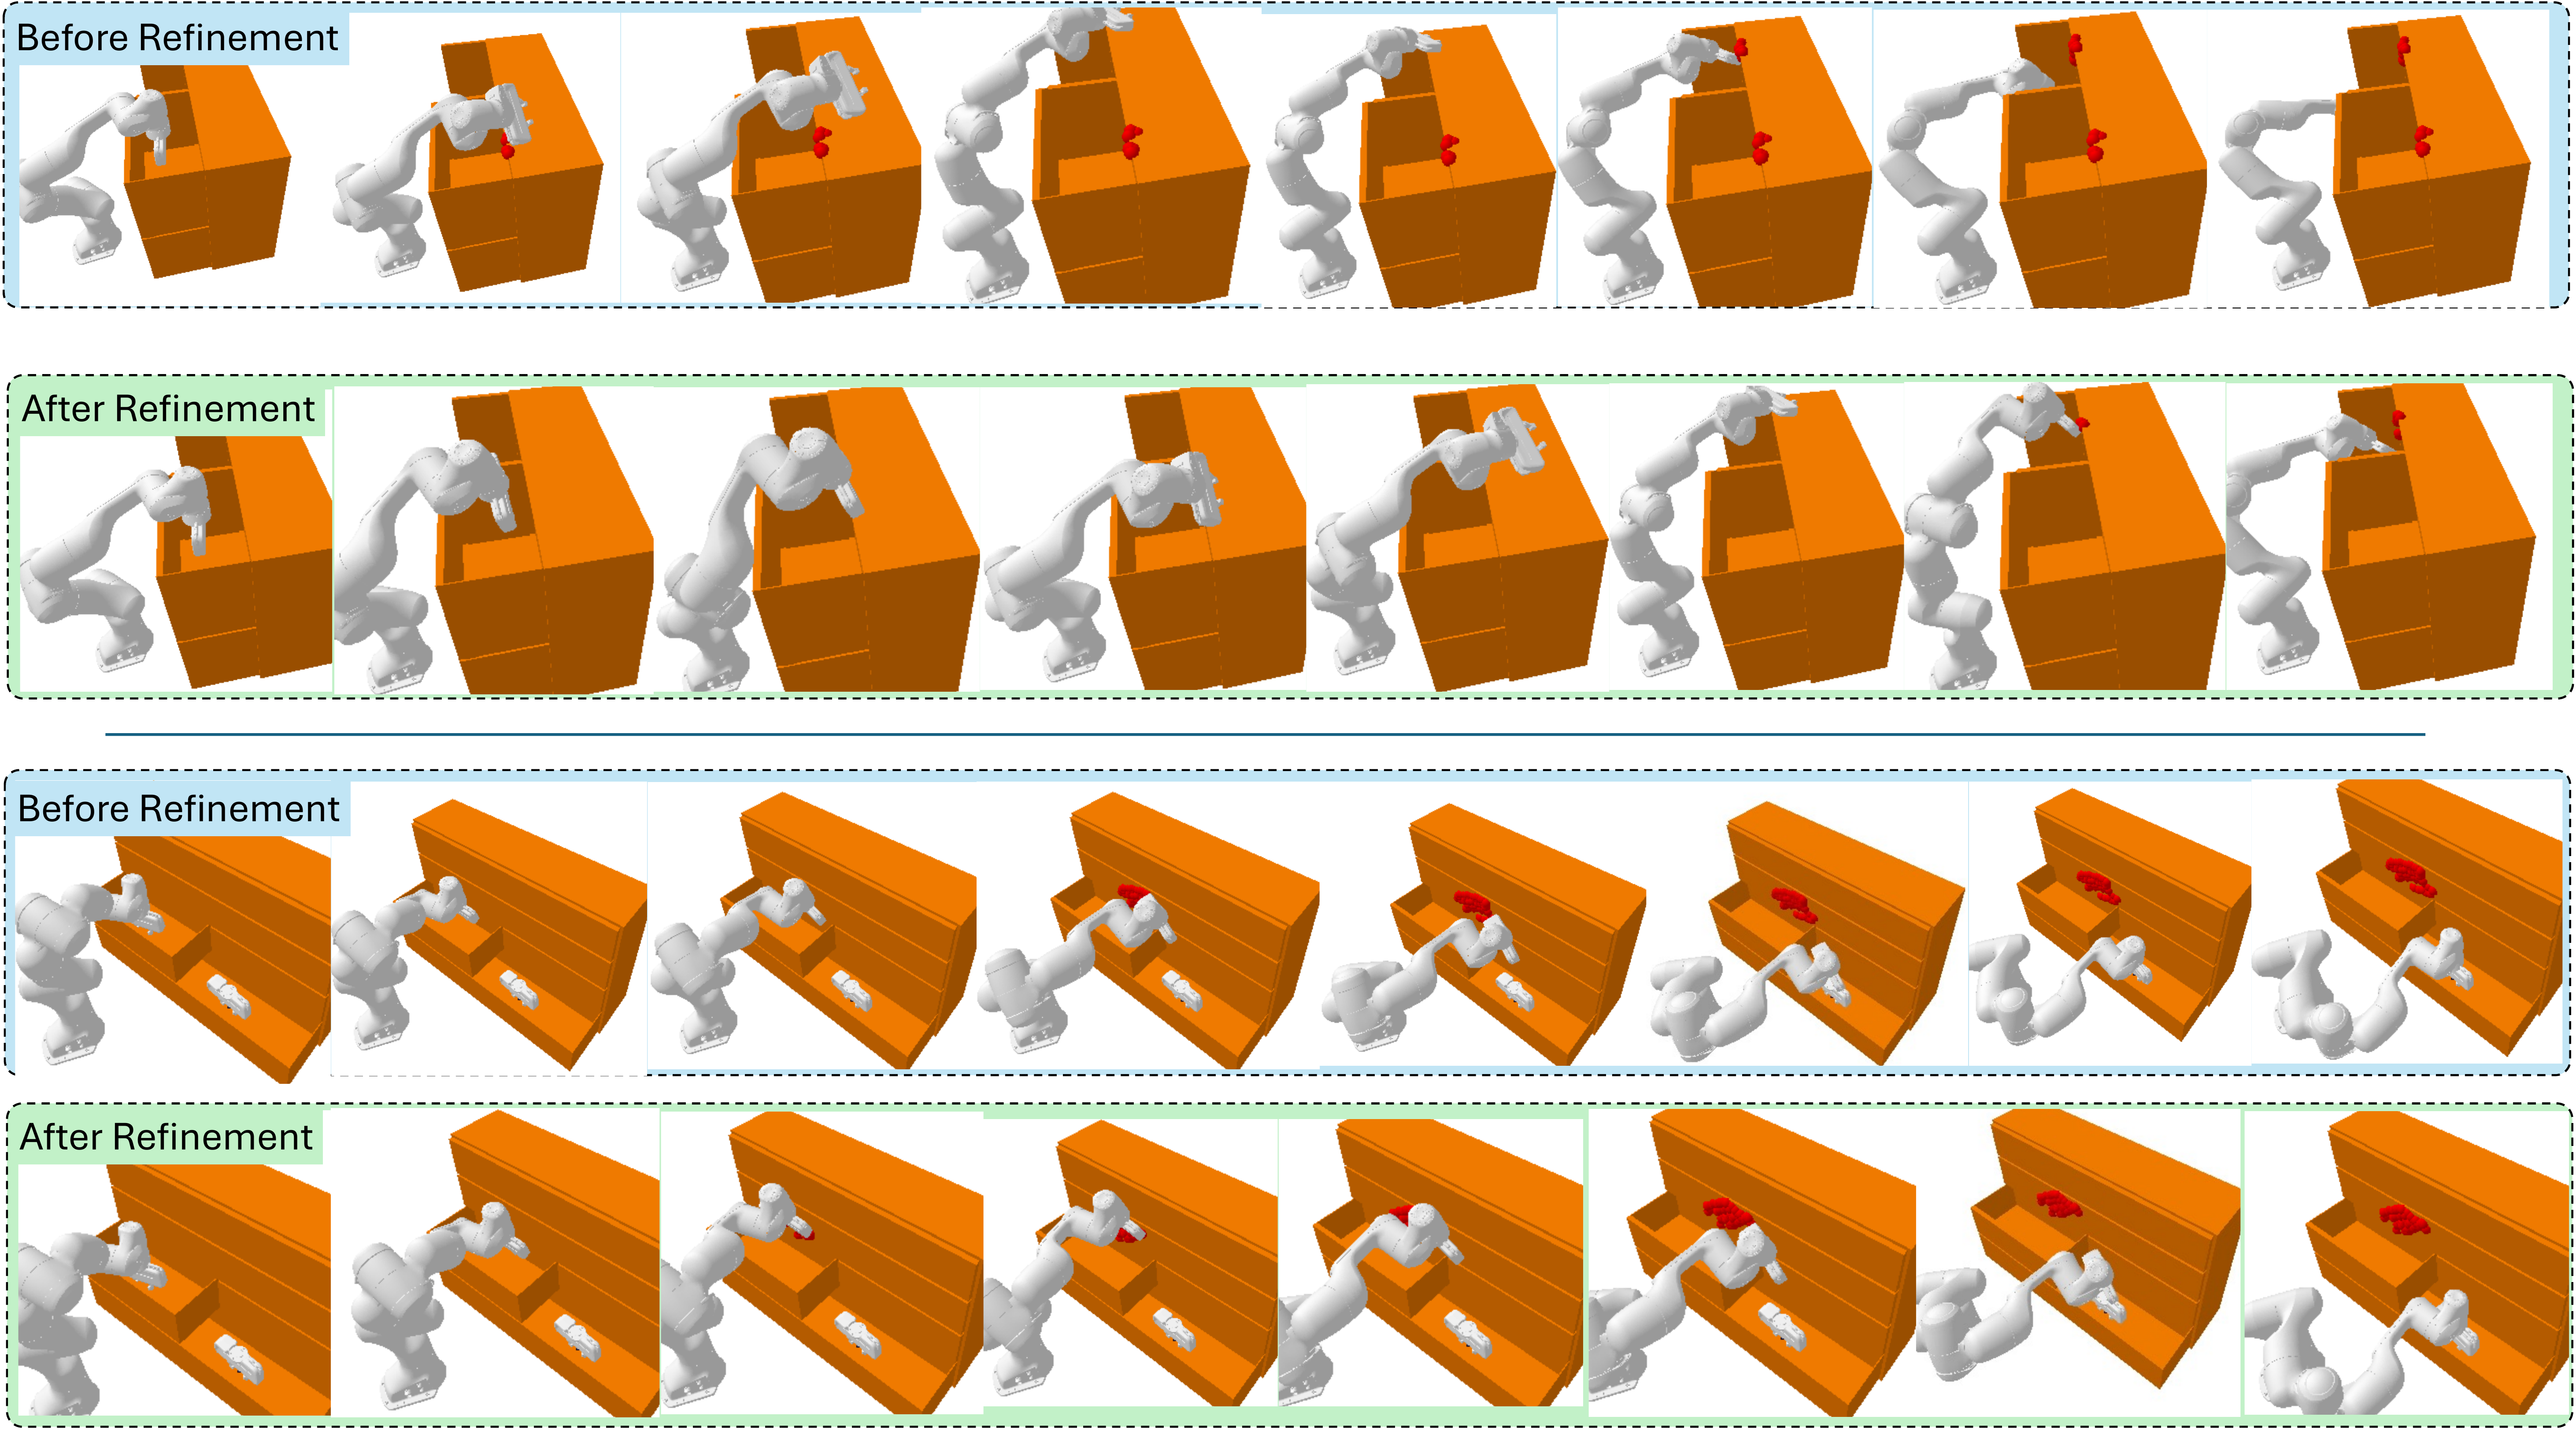} 
  \caption{\footnotesize{Failure scenarios. Some scenarios where our proposed approach (together with path refinement) fails to generate the complete motion without violating constraints.}}
  \label{fig:qualitative-results-app-01}
\end{figure}

\textbf{Failure Analysis:}
Figure~\ref{fig:qualitative-results-app-01} visualizes some scenes from \mpinetname Global test set where our model fails to perform well.
As can be seen in the above figure, in some scenarios (top-row) the model 
is able to repair a significant portion of the initial plan but fails to 
repair the latter part of the plan.
Thus, leading to few constraint violations in the latter part of the trajectory.
We believe running the plan refinement strategy multiple times may alleviate some of these failure scenarios.
Additionally, Figure~\ref{fig:qualitative-results-app-01} (bottom-row) also shows scenarios where our proposed approach together with low-level path refinement performs much more poorly. 
We believe this happens because in scenarios where the sub-goals and the reference trajectory points are quite poor. 
In such scenarios simply running the low-level plan refinement step is often  insufficient and still leads to many constraint violations (as seen in the above figure).

% Please add the following required packages to your document preamble:
% \usepackage{booktabs}
% \usepackage{graphicx}
\begin{table}[t]
\centering
\resizebox{0.7\textwidth}{!}{%
\begin{tabular}{@{}lll@{}}
\toprule
Low-level refinement & Cascaded Refinement & Low-Level Refinement + Guidance \\ \midrule
85.13 & 88.75 & 92.31 \\ \bottomrule \\
\end{tabular}%
}
\caption{\footnotesize{Comparison of our approach with different types of inference time adaptation. The first two sets of approaches Low-level refinement and Cascaded refinement do not require fully known geometry. However, the guidance approach assumes full geometric information about the scene and its objects.}}
\label{tab:app-cascaded-refinement}
\end{table}

Finally, we also report performance when we re-run our whole diffusion model
during the path refinement step (instead of only running the lower-level diffusion model).
Table~\ref{tab:app-cascaded-refinement} shows the results for the 3 different scenarios on \mpinetname Global dataset.
Specifically, our approach which \emph{only} uses low-level model refinement.
Our approach, but where we refine both high and low-level models. We refer to this as Cascaded Refinement. 
We note that for cascaded refinement we only use the high level policy if the number of states that are in collision exceed a specified threshold.
As can be seen in Table~\ref{tab:app-cascaded-refinement} while there is performance improvement in re-running the entire cascaded model (middle column),
it is less than the improvement we get when using collision guidance for the high level model.
This shows that the high-level diffusion model still struggles to generate paths in some of these scenes even with new start and goal configurations.
